# Supplementary material for: ASAP: Architecture Search, Anneal and Prune
Source: arXiv:1904.04123 source file (2019-10-10)
Supplement: Supplementary file 1 [file log_sum_exp_bounds.tex]

\label{log_sum_exp_bounds}
\begin{align*}
    x_{max}=& \\
    &\log\paren{e^{x_{max}}} \leq \\
    &\log\paren{\sum_{i=1}^N e^{x_{i}}} \\
    &\leq \log\paren{\sum_{i=1}^N e^{x_{max}}} \\
    &= \log\paren{N \cdot e^{x_{max}}} \\ 
    &\leq x_{max} + \log(N)
\end{align}
